# Supplementary material for: Adaptive Gradient Methods Can Be Provably Faster than SGD after Finite Epochs
Source: arXiv:2006.07037 source file (2020-06-12)
Supplement: Supplementary file 1 [file backup.tex]

\begin{lemma}
    \label{lem:G_trace_lower_bound}
    lem
\end{lemma}
\begin{proof}
    To simplify notations in the following proof, we set $s_i=\sum_{j=1}^m \left\|\grad f_{\sB_j^i}(\vx_j^i)\right\|^2$.
    Then, for each $s_i$, we have 
    \begin{equation}
        \label{ineq:G_trace_lower_bound_comp1}
        s_i = \sum_{j=1}^m \left\|\grad f_{\sB_j^i}(\vx_j^i)-\grad f_{\sB_j^i}(\vx_1^i) + \grad f_{\sB_j^i}(\vx_1^i)\right\|^2 \ge \sum_{j=1}^m\underbrace{\left[\left\|\grad f_{\sB_j^i}(\vx_1^i)\right\| - \left\|\grad f_{\sB_j^i}(\vx_j^i)-\grad f_{\sB_j^i}(\vx_1^i)\right\|\right]^2}_{T_1}.
    \end{equation}
    When the step size $\eta_{j,i}$ is small enough, i.e., 
    \begin{equation}
        \label{ineq:step_size_upper_bound}
        \begin{split}
            \eta_{.,i} \le \frac{\min_{k\in \sI_m}\left\|\grad f_{\sB_k^i}(\vx_1^i)\right\|}{2mL}\quad where\quad \eta_{j,i} = \eta_{.,i}\ \forall j\in\sI_m,
        \end{split}
    \end{equation}
    $T_1$ in \Eqref{ineq:G_trace_lower_bound_comp1} will be dominated by $\left\|\grad f_{\sB_j^i}(\vx_1^i)\right\|$, which means
    \begin{equation}
        \label{ineq:upper_bound_diff_gradients}
        \begin{split}
            & \left\|\grad f_{\sB_j^i}(\vx_j^i)-\grad f_{\sB_j^i}(\vx_1^i)\right\|^2 \mathop{\le}^{\circled{1}} L^2\left\|\vx_j^i - \vx_1^i\right\|^2 = L^2\left\|\sum_{k=1}^{j-1}\left(\vx_{k+1}^i - \vx_k^i\right)\right\|^2 \le L^2\left[\sum_{k=1}^{j-1}\left\|\vx_{k+1}^i - \vx_k^i\right\|\right]^2\\
            \mathop{\le}^{\circled{2}} & L^2(j-1)\left[\sum_{k=1}^{j-1}\left\|\vx_{k+1}^i - \vx_k^i\right\|^2\right] = L^2(j-1)\left[\underbrace{\sum_{k=1}^{j-1}\left\|\eta_{.,t}\mG^{-\frac{1}{2}}_{k,i}\grad f_{\sB_k^i}(\vx_k^i)\right\|^2}_{T_1}\right].
        \end{split}
    \end{equation}
    In \Eqref{ineq:upper_bound_diff_gradients}, $\circled{1}$ and $\circled{2}$ establish because of the $L-$Lipschitz continuous gradient assumption, the second point in Assumption~\ref{ass:comm_ass}, and the Cauchy-Schwarz inequality. Besides, each $k$ of $T_1$ in \Eqref{ineq:upper_bound_diff_gradients} satisfies
    \begin{equation}
        \label{ineq:T1_of_upper_bound_diff_gradients}
        \begin{split}
            &\left\|\mG^{-\frac{1}{2}}_{k,i}\grad f_{\sB_k^i}(\vx_k^i)\right\|^2 = \grad f^T_{\sB_k^i}(\vx_k^i)\mG^{-1}_{k,i}\grad f_{\sB_k^i}(\vx_k^i)\\
             = &\grad f^T_{\sB_k^i}(\vx_k^i)\left[\mG_{k-1,i} + \grad f_{\sB_k^i}(\vx_k^i)\grad f^T_{\sB_k^i}(\vx_k^i) \right]^{-1}\grad f_{\sB_k^i}(\vx_k^i)\\
             = &\grad f^T_{\sB_k^i}(\vx_k^i)\mG^{-1}_{k-1,i}\grad f_{\sB_k^i}(\vx_k^i) - \frac{\left\|f^T_{\sB_k^i}(\vx_k^i)\mG^{-1}_{k-1,i}\grad f_{\sB_k^i}(\vx_k^i)\right\|^2}{1+ f^T_{\sB_k^i}(\vx_k^i)\mG^{-1}_{k-1,i}\grad f_{\sB_k^i}(\vx_k^i)}\\
             = & \left(1+ f^T_{\sB_k^i}(\vx_k^i)\mG^{-1}_{k-1,i}\grad f_{\sB_k^i}(\vx_k^i)\right)^{-1} \le 1.
        \end{split}
    \end{equation}
    Thus, we submit \Eqref{ineq:T1_of_upper_bound_diff_gradients} backinto \Eqref{ineq:upper_bound_diff_gradients} to obtain
    \begin{equation}
        \label{ineq:upper_bound_diff_gradients_final}
        \begin{split}
            \left\|\grad f_{\sB_j^i}(\vx_j^i)-\grad f_{\sB_j^i}(\vx_1^i)\right\| \le L\left(j-1\right)\eta_{.,t}.
        \end{split}
    \end{equation}
    Combining \Eqref{ineq:upper_bound_diff_gradients_final}, \Eqref{ineq:step_size_upper_bound} with \Eqref{ineq:G_trace_lower_bound_comp1}, we have
    \begin{equation}
        \label{ineq:si_lower_bound}
        \begin{split}
            s_i\ge \frac{1}{4}\left[\sum_{j=1}^m \left\|\grad f_{\sB_j^i}(\vx_1^i)\right\|^2\right]\quad and\quad \mathbb{E}_{\sigma_i}\left[s_i\right]=\frac{1}{4}\sum_{j=1}^m\left(\mathbb{E}_{\sB_{j}^i}\left[\left\|\grad f_{\sB_j^i}(\vx_1^i)\right\|^2\right]\right).
        \end{split}
    \end{equation}
    With the symmetry of the permutation $\sigma_i$, there is $\mathbb{P}\left[\sB_1^i = \tilde{\sigma}\right]=\mathbb{P}\left[\sB_2^i = \tilde{\sigma}\right]=\ldots =\mathbb{P}\left[\sB_m^i = \tilde{\sigma}\right]$ for any specific subset $\tilde{\sigma} \subseteq \sI_m$ where $\left|\tilde{\sigma}\right| = \left|\sB_j^i\right|, \forall j\in\sI_m$.
    Thus, when the sample size of mini-batch $\left|\tilde{\sigma}\right|=n/m\le (n+1)/2$, the expectation $\mathbb{E}_{\sigma_i}\left[s_i\right]$ can be reformulated as
    \begin{equation}
        \label{ineq:exp_si_lower_bound}
        \begin{split}
            &\mathbb{E}_{\sigma_i}\left[s_i\right]=\frac{m}{4}\mathbb{E}_{\tilde{\sigma}}\left[\left\|\grad f_{\tilde{\sigma}}(\vx_1^i)\right\|^2\right] =\frac{m}{4}\mathbb{E}_{\tilde{\sigma}}\left[\left\|\grad f_{\tilde{\sigma}}(\vx_1^i)-\mathbb{E}_{\tilde{\sigma}}\left[\grad f_{\tilde{\sigma}}(\vx_1^i)\right]+\mathbb{E}_{\tilde{\sigma}}\left[\grad f_{\tilde{\sigma}}(\vx_1^i)\right]\right\|^2\right]\\
            = & \frac{m}{4}\left[\mathbb{E}_{\tilde{\sigma}}\left[\left\|\grad f_{\tilde{\sigma}}(\vx_1^i)-\mathbb{E}_{\tilde{\sigma}}\left[\grad f_{\tilde{\sigma}}(\vx_1^i)\right]\right\|^2\right] + \mathbb{E}_{\tilde{\sigma}}\left[\left\|\mathbb{E}_{\tilde{\sigma}}\left[\grad f_{\tilde{\sigma}}(\vx_1^i)\right]\right\|^2\right]\right]\\
            \ge &\frac{m}{4}\mathbb{E}_{\tilde{\sigma}}\left[\left\|\grad f_{\tilde{\sigma}}(\vx_1^i)-\mathbb{E}_{\tilde{\sigma}}\left[\grad f_{\tilde{\sigma}}(\vx_1^i)\right]\right\|^2\right] \mathop{=}^{\circled{1}} \frac{m}{4}\cdot \frac{c^2_{\sigma}m}{n} \cdot \left(1-\frac{n/m-1}{n-1}\right) \ge \frac{c^2_{\sigma}m^2}{8n},
        \end{split}
    \end{equation}
    where $\circled{1}$ establish because of the property of sampling without replacement\cite{}. 
    Besides, for any $i\in\sI_m$, we have $s_i\in \left[0,mG^2\right]$.
    According to Lemma~\ref{lem:hoeffding_s_inequality}, we have
    \begin{equation}
        \label{ineq:s_i_hoeffding_bound}
        \begin{split}
            \mathbb{P}\left[\rs_i-\frac{c^2_{\sigma}m^2}{8n}\le -\frac{c^2_{\sigma}m^2}{16n}\right] \le \mathbb{P}\left[\rs_i-\mathbb{E}\left[\rs_i\right]\le -\frac{c^2_{\sigma}m^2}{16n}\right]\le \exp\left(-\frac{c^2_{\sigma}m^2}{128n^2G^4}\right).
        \end{split}
    \end{equation}
    That is to say, $s_i\ge \frac{c^2_{\sigma}m^2}{16n}$ establishes with probability at least $1-\exp\left(-\frac{c^2_{\sigma}m^2}{128n^2G^4}\right)$. 
    %Submitting \Eqref{ineq:exp_si_lower_bound} backinto \Eqref{ineq:trG_norm_version}, we obtain
    %\begin{equation}
    %    \label{ineq:trG_norm_version_final}
    %    \begin{split}
    %        \mathbb{E}\left[tr(\mG_{m,t})\right] = \sum_{i=1}^t \mathbb{E}\left[s_i\right] + \delta_{m,t} \ge \sum_{i=1}^t \mathbb{E}\left[s_i\right] \ge \frac{tc^2_{\sigma}m^2}{4n}.
    %    \end{split}
    %\end{equation}
    %Hence, when $\delta_{m,t}\le \sqrt{mt}G$, we %complete the proof with
    %\begin{equation}
    %    \label{lem:G_trace_lower_bound_final}
    %    \begin{split}
    %        \mathbb{E}\left[tr\left(\mG_{m,t}\right)^{\frac{1}{2}}\right] = \mathbb{E}\left[\frac{tr\left(\mG_{m,t}\right)}{tr\left(\mG_{m,t}\right)^{\frac{1}{2}}}\right] \mathop{\ge}^{\circled{1}} \frac{\mathbb{E}\left[tr\left(\mG_{m,t}\right)\right]}{\sqrt{mt}G+\delta_{m,t}} \ge \frac{c^2_{\sigma}m^{1.5}t^{0.5}}{8nG}.
    %    \end{split}
    %\end{equation}
    %It should be notice that we have $\circled{1}$ because of the gradient upper bound assumption, the forth point in Assumption~\ref{ass:comm_ass}. 
\end{proof}
\begin{assumption}
    \label{ass:kappa_bounded_ass}
    We assume $\mH_{m,t}$ is full rank, and the condition number of $\mH_{m,t}\mH_{m,t}^T$ satisfies
    \begin{equation}
        \kappa_{m,t}\coloneqq \frac{\lambda_{\rm{max}}\left(\mH_{m,t}\mH_{m,t}^T\right)}{\lambda_{\rm{min}}\left(\mH_{m,t}\mH_{m,t}^T\right)}\le c_{\kappa}
    \end{equation}
    where $c_{\kappa}$ is a constant which will not decrease when the number of epoch increasing. 
\end{assumption}


\begin{proof}
    We denote $\sS_+^{d\times d}$ as the positive-definite matrix set with size $d\times  d$. 
    According to the fact $\mG_{m,i}\in \sS_+^{d\times d}$, if the hyper-parameter $\delta_{m,i}\le imG^2$, then
    \begin{equation}
        \label{ineq:tr_root_psd_upper_bound}
        \begin{aligned}[b]
            \left[tr\left(\mG^{\frac{1}{2}}_{m,i}\right)\right]^2 = &\left[\sqrt{\lambda_1\left(\mG_{m,i}\right)}+ \sqrt{\lambda_2\left(\mG_{m,i}\right)}+\ldots+\sqrt{\lambda_d\left(\mG_{m,i}\right)}\right]^2\\
            \le & \left[\lambda_1\left(\mG_{m,i}\right) + \lambda_2\left(\mG_{m,i}\right)+\ldots + \lambda_d\left(\mG_{m,i}\right)\right]\cdot d = tr\left(\mG_{m,i}\right) \cdot d\\
            \mathop{\le}^{\circled{1}} &\left[imG^2 + \delta_{m,i}\right]\cdot d \le 2imG^2d,
        \end{aligned}
    \end{equation}
    where $\circled{1}$ establishes because of the definition of matrix $\mG_{m,i}$:
    \begin{equation}
        \label{ineq:trace_G_upper_bound}
        tr\left(\mG_{m,i}\right) = \sum_{j=1}^{i}\sum_{k=1}^m \left\|\grad f_{\sB_k^j}(\vx_k^j)\right\|^2 + \delta_{m,i} \le imG^2+\delta_{m,i}.
    \end{equation}
    Besides, when $\delta_{m,i}$ is increasing with $i$'s growth, the matrix $\left(\mG_{m,i}-\mG_{m,i-1}\right) \in \sS_+^{d\times d}$. 
    Hence,
    \begin{equation}
        \label{ineq:tr_root_psd_lower_bound}
        \begin{aligned}[b]
            &\lambda_{min}\left[\left(\mG_{m,i}-\mG_{m,i-1}\right)^{\frac{1}{2}}\right] = \lambda_{min}\left[\left(\sum_{j=1}^m \grad f_{\sB_j^{i}}(\vx_j^{i})\grad f^T_{\sB_j^{i}}(\vx_j^{i})+\frac{\delta_{m,i} - \delta_{m,i-1}}{d}\mI\right)^{\frac{1}{2}}\right]\\
            \ge &\sqrt{\frac{\delta_{m,i} - \delta_{m,i-1}}{d}}.
        \end{aligned}
    \end{equation}
    Combining Eq.~\ref{ineq:tr_root_psd_lower_bound} with Eq.~\ref{ineq:tr_root_psd_upper_bound}, set
    \begin{equation}
        \label{eq:beta_i_selection}
        \begin{split}
            \beta_{i} = \sqrt{\frac{\delta_{m,i}-\delta_{m,i-1}}{2imG^2d^2}},
        \end{split}
    \end{equation}
    we have
    \begin{equation}
        \label{ineq:order_sufficient_condition_1}
        \begin{split}
            \beta_{i}\lambda_{max}\left(\mG^{\frac{1}{2}}_{m,i}\right)\le \beta_{i}tr\left(\mG^{\frac{1}{2}}_{m,i}\right) \le \lambda_{min}\left[\left(\mG_{m,i}-\mG_{m,i-1}\right)^{\frac{1}{2}}\right].
        \end{split}
    \end{equation}
    With the fact $\mG^{\frac{1}{2}}_{m,i}, \left(\mG_{m,i}-\mG_{m,i-1}\right)^{\frac{1}{2}}\in \sS_+^{d\times d}$, there is 
    \begin{equation}
        \label{ineq:order_sufficient_condition_2}
        \begin{aligned}[b]
            & \beta_{i}\mG^{\frac{1}{2}}_{m,i} \preceq \left(\mG_{m,i}-\mG_{m,i-1}\right)^{\frac{1}{2}} \mathop{\Rightarrow}^{\circled{1}} \beta_{i}\left(\mG_{m,i}-\mG_{m,i-1}\right)^{-\frac{1}{2}} \preceq \mG^{-\frac{1}{2}}_{m,i}\\
            \mathop{\Rightarrow}^{\circled{2}} & \left[\sum_{j=1}^m \grad f_{\sB_j^i}(\vx_j^i)\right]^T\left[\beta_{i}\left(\mG_{m,i}-\mG_{m,i-1}\right)^{-\frac{1}{2}}\right]\left[\sum_{j=1}^m \grad f_{\sB_j^i}(\vx_j^i)\right]\\
            &\le \left[\sum_{j=1}^m \grad f_{\sB_j^i}(\vx_j^i)\right]^T\mG^{-\frac{1}{2}}_{m,i}\left[\sum_{j=1}^m \grad f_{\sB_j^i}(\vx_j^i)\right],
        \end{aligned}
    \end{equation}
    where we have $\circled{1}$ and $\circled{2}$ due to Lemma~\ref{lem:matrix_inverse_positive_definite_lemma} and Lemma~\ref{lem:conjugate_rule}, respectively.
\end{proof}

\begin{lemma}
    \label{lem:kappa_bounded_lemma}
    Suppose the Assumption~\ref{ass:comm_ass} and Assumption~\ref{ass:H_full_column_rank_ass} hold and $\mH_{m,t}$ defined as \Eqref{eq:H_matrix_definition}, we have
    \begin{equation}
        \label{ineq:kappa_bounded_sum}
        \frac{\lambda_{\rm{max}}\left(\mH^T_{m,t}\mH_{m,t}\right)}{\lambda_{\rm{min}}\left(\mH^T_{m,t}\mH_{m,t}\right)}\le 2G^{m+2}m^{m+1} \coloneqq c_{\kappa}
    \end{equation}
\end{lemma}
\begin{proof}
    According to Theorem 1 in \cite{guggenheimer1995simple}, we have
    \begin{equation}
        \label{ineq:lambda_min_lower_bound}
        \frac{\lambda_{\rm{max}}\left(\mH^T_{m,t}\mH_{m,t}\right)}{\lambda_{\rm{min}}\left(\mH^T_{m,t}\mH_{m,t}\right)} = \kappa_2\left(\mH^T_{m,t}\mH_{m,t}\right)\le 2\left|\det \left(\mH^T_{m,t}\mH_{m,t}\right)\right|\left\|\mH^T_{m,t}\mH_{m,t}\right\|_Fm^m.
    \end{equation}
    With gradient norm bound, the forth point of Assumption~\ref{ass:comm_ass}, there is 
    \begin{equation}
        \label{ineq:det_upper_bound}
        \begin{split}
            \det \left(\mH^T_{m,t}\mH_{m,t}\right) \mathop{\le}^{\circled{1}} \prod_{i=1}^m \left(\left[
                \begin{matrix}
                    \grad f^T_{\sB_t^1}(\vx_t^1)\\
                    \grad f^T_{\sB_t^2}(\vx_t^2)\\
                    \ldots \\
                    \grad f^T_{\sB_t^m}(\vx_t^m)
                \end{matrix}
            \right]
            \left[\grad f_{\sB_t^1}(\vx_t^1), \grad f_{\sB_2^t}(\vx_2^t),\ldots, \grad f_{\sB_m^t}(\vx_m^t)\right]\right)_{i,i}\le G^m,
        \end{split}
    \end{equation}
    where $\circled{1}$ is eatablished because of Lemma~\ref{lem:hadamard_inequality}.
    Besides, with the property of F-norm, we have
    \begin{equation}
        \label{ineq:F_norm_upper_bound}
        \begin{split}
            \left\|\mH^T_{m,t}\mH_{m,t}\right\|_F\le \left\|\mH_{m,t}\right\|_F^2\le \sum_{i=1}^m \left\|\grad f_{\sB_t^i}(\vx_t^i)\right\|^2\le mG^2
        \end{split}
    \end{equation}
    Combining Eq.~\ref{ineq:F_norm_upper_bound}, Eq.~\ref{ineq:det_upper_bound} and Eq.~\ref{ineq:lambda_min_lower_bound}, we then obtain
    \begin{equation}
        \label{ineq:kappa_bound_fin}
        \begin{split}
            \kappa_2\left(\mH^T_{m,t}\mH_{m,t}\right)\le 2G^{m+2}m^{m+1}
        \end{split}
    \end{equation}
    for any $t$ to complete the proof. 
    It should be notice that we have $c_\kappa\le 2G$ when $G\le 1/m$, and the gradient norm upper bound can be reduced when the objective function is multiplied by a tiny constant independent with $T$ and $\epsilon$.
    Hence, we denote the constant $c_\kappa$ as the upper bound of the condition number of $\mH^T_{m,t}\mH_{m,t}$ for convenience.
\end{proof}

\begin{lemma}[Hadamard's inequality]
    \label{lem:hadamard_inequality}
    A positive-semidefinite matrix $\mM\in\mathbb{C}^{d\times d}$ can be written as $\mN^*\mN$, where $\mN^*$ denotes the conjugate transpose of $\mN$. Then
    \begin{equation}
        \label{ineq:hadamard_inequality}
        \begin{aligned}[b]
            \det\left(\mM\right)  = \det\left(\mN\right)^2 \le \prod_{i=1}^d\left\|\vv_i\right\|^2 = \prod_{i=1}^d \mM_{ii},
        \end{aligned}
    \end{equation}
    where $\vv_i$ and $\mM_{ii}$ denote the $i$-th column vector of $\mN$ and the $i$-th diagonal element of $\mM$.
\end{lemma}

\begin{lemma}
    Suppose the Assumption~\ref{ass:comm_ass} and Assumption~\ref{ass:H_full_column_rank_ass} hold and $\mH_{m,t}$ is defined as Eq.~\ref{eq:H_matrix_definition}, we have
    \begin{equation}
        \label{ineq:condition_number_upper_bound_pre}
        \begin{aligned}[b]
            \frac{\lambda_{max}\left(\mH^T_{m,t}\mH_{m,t}\right)}{\lambda_{min}\left(\mH^T_{m,t}\mH_{m,t}\right)} \le \frac{16nG^2}{c_{\sigma}^2} \coloneqq c_{\kappa}
        \end{aligned}
    \end{equation}
    with probability at least $1-\exp\left(-\frac{c^2_{\sigma}m^2}{32n^2G^4}\right)$.
\end{lemma}
\begin{proof}
    To obtain the condition number of $\mH^T_{m,t}\mH_{m,t}$, we firstly provide the upper bound of $\lambda_{max}\left(\mH^T_{m,t}\mH_{m,t}\right)$.
    \begin{equation}
        \label{ineq:lambda_max_upper_bound}
        \begin{aligned}
            \lambda_{max}\left(\mH^T_{m,t}\mH_{m,t}\right) \le tr\left(\mH^T_{m,t}\mH_{m,t}\right)  = \sum_{j=1}^m \left\|\grad f_{\sB_j^t}\left(\vx_j^t\right)\right\|^2\le mG^2.
        \end{aligned}
    \end{equation}
    Then, we provide the lower bound of $\lambda_{min}\left(\mH^T_{m,t}\mH_{m,t}\right)$.
    According to the fact that non-zero eigenvalues of $\mH^T_{m,t}\mH_{m,t}$ and $\mH_{m,t}\mH^T_{m,t}$ have the same algrebraic multiplicity. 
    That is to say, $\lambda_{min}\left(\mH^T_{m,t}\mH_{m,t}\right) = \lambda_{min}\left(\mH_{m,t}\mH_{m,t}^T\right)$.
    We construct a vector sequence, i.e., $\vv_i = \grad f_{\sB^t_{l_i}}(\vx^t_{l_i}), i\in \sI_m$, where $\left\|\vv_i\right\|\ge \left\|\vv_j\right\|$ if $i<j$.
    That is to say, $\vv_i$ denotes the $i$-th longest mini-batch gradient in the $t$-th epoch.
    With the sequence $\left\{\vv_i\right\}_{i=1}^m$, we define $\mV_{i}  = \mV_{i-1} + \vv_i\vv_i^T = \sum_{j=1}^i \vv_i\vv_i^T$, and $\mV_m = \mH_{m,t}\mH_{m,t}^T$.
    Hence, we have
    \begin{equation}
        \label{ineq:lambda_min_lower_bound_1}
        \begin{aligned}
            \lambda_{min}\left(\mH_{m,t}\mH_{m,t}^T\right) = \lambda_{min}\left(\mV_m\right) \mathop{\ge}^{\circled{1}} \lambda_{min}\left(\mV_{m-1}\right) \mathop{\ge}^{\circled{1}} \ldots \ge \lambda_{min}\left(\mV_1\right) = \left\|\vv_1\right\|^2,
        \end{aligned}
    \end{equation}
    where $\circled{1}$ follows from Corollary~\ref{cor:welys_inequality}.
    According to our definition, we have
    \begin{equation}
        \label{ineq:lambda_min_lower_bound_2}
        \begin{aligned}
            \left\|\vv_1\right\|^2 \ge \frac{1}{m}\sum_{j=1}^m \left\|\grad f_{\sB_j^t}(\vx_j^t)\right\|^2 \mathop{\ge}^{\circled{1}} \frac{c_\sigma^2m}{16n}
        \end{aligned}
    \end{equation}
    with probability at least $1-\exp\left(-\frac{c^2_{\sigma}m^2}{32n^2G^4}\right)$.
    Notice that $\circled{1}$ is established due to Lemma~\ref{lem:G_trace_lower_bound}.
    Then, we have
    \begin{equation}
        \label{ineq:condition_number_upper_bound}
        \begin{aligned}[b]
            \frac{\lambda_{max}\left(\mH^T_{m,t}\mH_{m,t}\right)}{\lambda_{min}\left(\mH^T_{m,t}\mH_{m,t}\right)} \le \frac{\lambda_{max}\left(\mH^T_{m,t}\mH_{m,t}\right)}{\left\|\vv_1\right\|^2}\mathop{\le}^{\circled{1}}  \frac{16nG^2}{c_{\sigma}^2}
        \end{aligned}
    \end{equation}
    with probability at least $1-\exp\left(-\frac{c^2_{\sigma}m^2}{32n^2G^4}\right)$.
    The proof is completed.
\end{proof}

\begin{lemma}[Weyl's inequality in matrix theory]
    \label{lem:welys_inequality}
    Let a matrix $\mM$ be formulated as $\mM = \mH + \mP$, where any two of $\mM, \mH$ and $\mP$ are $d$ by $d$ Hermitian matrices.
    If $\mM$ has eigenvalues $\lambda_1\left(\mM\right)\ge \lambda_2\left(\mM\right) \ge \ldots \ge \lambda_d\left(\mM\right)$,
    and $\mH$ has eigenvalues $\lambda_1\left(\mH\right)\ge \lambda_2\left(\mH\right) \ge \ldots \ge \lambda_d\left(\mH\right)$, and $\mP$ has eigenvalues $\lambda_1\left(\mP\right)\ge \lambda_2\left(\mP\right) \ge \ldots \ge \lambda_d\left(\mP\right)$.
    The following inequalities hold for $i=1,2,\ldots, d$:
    \begin{equation}
        \label{ineq:welys_inequality_1}
        \begin{aligned}
            \lambda_i\left(\mH\right)+\lambda_d\left(\mP\right) \le \lambda_i\left(\mM\right) \le \lambda_i\left(\mH\right)+\lambda_1\left(\mP\right)
        \end{aligned}
    \end{equation}
\end{lemma}
\begin{corollary}[Weyl's inequality in matrix theory]
    \label{cor:welys_inequality}
    Let $\mM$ be a real symmetric matrix whose eigenvalues satisfy $\lambda_1\left(\mM\right)\ge \lambda_2\left(\mM\right) \ge \lambda_k \left(\mM\right)$.
    For any real vector $\vv$, the following inequality holds
    \begin{equation}
        \label{ineq:welys_inequality_2}
        \begin{aligned}
            \lambda_k\left(\mM\right) \le \lambda_{min}\left(\mM + \vv\vv^T\right) \le \lambda_{k-1}\left(\mM\right).
        \end{aligned}
    \end{equation}
\end{corollary}

\begin{lemma}
    \label{lem:comp_G_lambda_bound}
    In \adagrad, suppose that the Assumption~\ref{ass:comm_ass} hold, and the perturbation $\delta_{i,t}$ is no decreasing. For any $1\le i \le m$, we have
    \begin{equation}
        \label{ineq:comp_G_lambda_bound}
        0\preceq \mG_{m,t}^{\frac{1}{4}}\mG_{i,t}^{-\frac{1}{2}}\mG_{m,t}^{\frac{1}{4}}-\mI \preceq \sqrt{\frac{\Delta_{i,t}}{\lambda_{min}\left(\mG_{i,t}\right)}}\mI,
    \end{equation}
    where $\Delta_{i,t} \coloneqq \left[(m-i)G^2+ \left(\delta_{m,t}-\delta_{i,t}\right)\right]$.
\end{lemma}
\begin{proof}
    According to the difinition of $\mG_{m,t}$, we have
    \begin{equation}
        \label{ineq:G_matrix_upperbound}
        \begin{aligned}[b]
            \mG_{m,t} =& \mG_{i,t}+\sum_{j=i+1}^m\grad f_{\sB_j^t}(\vx_j^t)\grad f^T_{\sB_j^t}(\vx_j^t) + \frac{\delta_{m,t}-\delta_{i,t}}{m}\mI \\
            \preceq &\mG_{i,t}+\lambda_{max}\left(\sum_{j=i+1}^m\grad f_{\sB_j^t}(\vx_j^t)\grad f^T_{\sB_j^t}(\vx_j^t) + \frac{\delta_{m,t}-\delta_{i,t}}{m}\mI\right)\cdot \mI\\
            \preceq & \mG_{i,t} + \lambda_{max}\left(\sum_{j=i+1}^m\grad f_{\sB_j^t}(\vx_j^t)\grad f^T_{\sB_j^t}(\vx_j^t)\right) +  \frac{\delta_{m,t}-\delta_{i,t}}{m}\cdot \mI\\
            \mathop{\preceq}^{\circled{1}} &\mG_{i,t} + tr\left(\sum_{j=i+1}^m\grad f_{\sB_j^t}(\vx_j^t)\grad f^T_{\sB_j^t}(\vx_j^t)\right)\cdot \mI + \frac{\delta_{m,t}-\delta_{i,t}}{m}\mI\\
            \mathop{\preceq}^{\circled{2}} &\mG_{i,t}+\left[(m-i)G^2+ \left(\delta_{m,t}-\delta_{i,t}\right)\right]\mI,
        \end{aligned}
    \end{equation}
    where $\circled{1}$ follows from the positive-definite property of the matrix $\mG_{m,t}-\mG_{i,t}$ and $\circled{2}$ follows from 
    the gradient bounded assumption, i.e., the forth item of Assumption~\ref{ass:comm_ass}.
    Thus, if $\mG_{i,t} = \mP_{i,t}\mSigma_{i,t}\mP_{i,t}^T$, which means the SVD of the matrix $\mG_{i,t}$, $\mG_{m,t}$ satisfies
    \begin{equation}
        \label{ineq:G_matrix_upperbound_2}
        \begin{split}
            \mG_{m,t}\preceq \mG_{i,t}+\left[(m-i)G^2+ \left(\delta_{m,t}-\delta_{i,t}\right)\right]\mI = \mP_{i,t}\left[\mSigma_{i,t} + \Delta_{i,t}\mI\right]\mP_{i,t}^T.
        \end{split}
    \end{equation}
    According to Lemma~\ref{lem:matrix_root_positive_definite_lemma} and Lemma~\ref{lem:matrix_inverse_positive_definite_lemma}, with $\mG_{m,t}\succeq \mG_{i,t}$, we have $\mG_{i,t}^{-\frac{1}{2}} \succeq \mG_{m,t}^{-\frac{1}{2}}$.
    Besides, we have
    \begin{equation}
        \label{ineq:square_term_lower_bound}
        \begin{split}
            \mG_{m,t}^{\frac{1}{4}}\mG_{i,t}^{-\frac{1}{2}}\mG_{m,t}^{\frac{1}{4}}\succeq \mG_{m,t}^{\frac{1}{4}}\mG_{m,t}^{-\frac{1}{2}}\mG_{m,t}^{\frac{1}{4}} = \mI
        \end{split}
    \end{equation}
    because of Lemma~\ref{lem:conjugate_rule}.
    According to Jacobson's lemma in operator theory,  for any two bounded operators $\mA$ and $\mB$ on a Hilbert space $\sH$, the non-zero points of the spectrum of $\mA\mB$ coincide with those of the spectrum of $\mB\mA$.
    Set $\mA = \mG_{m,t}^{\frac{1}{4}}\mG_{i,t}^{-\frac{1}{4}}$ and $\mB = \mG_{i,t}^{-\frac{1}{4}}\mG_{m,t}^{\frac{1}{4}}$, we have
    \begin{equation}
        \label{ineq:square_term_upper_bound}
        \begin{aligned}[b]
            & \lambda_{max}\left(\mG_{m,t}^{\frac{1}{4}}\mG_{i,t}^{-\frac{1}{2}}\mG_{m,t}^{\frac{1}{4}}\right) = \lambda_{max}\left(\mG_{i,t}^{-\frac{1}{4}}\mG_{m,t}^{\frac{1}{2}}\mG_{i,t}^{-\frac{1}{4}}\right)\\
            \mathop{\le}^{\circled{1}} & \lambda_{max}\left(\mG_{i,t}^{-\frac{1}{4}}\left[\mP_{i,t}\left[\mSigma_{i,t} + \Delta_{i,t}\mI\right]\mP_{i,t}^T\right]^{\frac{1}{2}}\mG_{i,t}^{-\frac{1}{4}}\right)\\
            = &\lambda_{max}\left(\mP_{i,t}\left[\mSigma_{i,t} + \Delta_{i,t}\mI\right]^{\frac{1}{2}}\mSigma_{i,t}^{-\frac{1}{2}}\mP^T_{i,t}\right) = \sqrt{\frac{\lambda_{min}\left(\mG_{i,t}\right)+ \Delta_{i,t}}{\lambda_{min}\left(\mG_{i,t}\right)}},
        \end{aligned}
    \end{equation} 
    where $\circled{1}$ follows from Eq.~\ref{ineq:G_matrix_upperbound_2}, Lemma~\ref{lem:matrix_root_positive_definite_lemma} and Lemma~\ref{lem:conjugate_rule}.
    Combining Eq.~\ref{ineq:square_term_lower_bound} with Eq.~\ref{ineq:square_term_upper_bound}, we obtain
    \begin{equation}
        \label{ineq:square_term_bound}
        \begin{split}
            0\preceq \mG_{m,t}^{\frac{1}{4}}\mG_{i,t}^{-\frac{1}{2}}\mG_{m,t}^{\frac{1}{4}}-\mI \preceq \left[\sqrt{\frac{\lambda_{min}\left(\mG_{i,t}\right)+ \Delta_{i,t}}{\lambda_{min}\left(\mG_{i,t}\right)}}-1\right]\mI \mathop{\preceq}^{\circled{1}} \sqrt{\frac{\Delta_{i,t}}{\lambda_{min}\left(\mG_{i,t}\right)}}\mI,
        \end{split}
    \end{equation}
    where $\circled{1}$ follows from the fact $\sqrt{c+1}\le \sqrt{c}+1, \forall c\ge 0$.
    Hence, we complete the proof.
\end{proof}

\begin{equation}
    \label{ineq:descent_constant_lower_bound}
    \begin{aligned}[b]
        &\left\|\vx_{k+1}^i - \vx_k^i\right\|=\left\|\eta_{.,i}\mG_{k,i}^{-\frac{1}{2}}\grad f_{\sB_k^i}(\vx_k^i)\right\|=\eta_{.,t}\sqrt{\grad f^T_{\sB_k^i}(\vx_k^i) \mG_{k,i}^{-1}\grad f_{\sB_k^i}(\vx_k^i)}\\
        = &\eta_{.,i}\sqrt{\grad f^T_{\sB_k^i}(\vx_k^i)\left[\mG_{k-1,i}+ \frac{\delta_{k,i}-\delta_{k-1,i}}{m} \cdot \mI + \grad f_{\sB_k^i}(\vx_k^i)\grad f^T_{\sB_k^i}(\vx_k^i) \right]^{-1}\grad f_{\sB_k^i}(\vx_k^i)}\\
        \le & \eta_{.,i}\sqrt{\grad f^T_{\sB_k^i}(\vx_k^i)\left[\mG_{k-1,i}+ \grad f_{\sB_k^i}(\vx_k^i)\grad f^T_{\sB_k^i}(\vx_k^i) \right]^{-1}\grad f_{\sB_k^i}(\vx_k^i)}\\
         \mathop{=}^{\circled{1}} &\eta_{.,i}\sqrt{\grad f^T_{\sB_k^i}(\vx_k^i)\mG^{-1}_{k-1,i}\grad f_{\sB_k^i}(\vx_k^i) - \frac{\left\|f^T_{\sB_k^i}(\vx_k^i)\mG^{-1}_{k-1,i}\grad f_{\sB_k^i}(\vx_k^i)\right\|^2}{1+ f^T_{\sB_k^i}(\vx_k^i)\mG^{-1}_{k-1,i}\grad f_{\sB_k^i}(\vx_k^i)}}\\
         = & \eta_{.,i}\left(1+ f^T_{\sB_k^i}(\vx_k^i)\mG^{-1}_{k-1,i}\grad f_{\sB_k^i}(\vx_k^i)\right)^{-\frac{1}{2}} \le \eta_{.,i}.
    \end{aligned}
\end{equation}
\begin{equation}
    \label{ineq:T2_for_SD_component1}
    \begin{aligned}[b]
        &\grad f^T_{\sB_i^t}(\vx_i^t) \left(\mG_{m,t}^{-\frac{1}{2}}-\mG_{i,t}^{-\frac{1}{2}}\right)\mG_{m,t}^{\frac{1}{2}}\left(\mG_{m,t}^{-\frac{1}{2}}-\mG_{i,t}^{-\frac{1}{2}}\right)\grad f_{\sB_i^t}(\vx_i^t)\\
        =&\grad f^T_{\sB_i^t}(\vx_i^t)\mG_{m,t}^{-\frac{1}{4}}\mG_{m,t}^{\frac{1}{4}} \left(\mG_{m,t}^{-\frac{1}{2}}-\mG_{i,t}^{-\frac{1}{2}}\right)\mG_{m,t}^{\frac{1}{2}}\left(\mG_{m,t}^{-\frac{1}{2}}-\mG_{i,t}^{-\frac{1}{2}}\right)\mG_{m,t}^{\frac{1}{4}}\mG_{m,t}^{-\frac{1}{4}}\grad f_{\sB_i^t}(\vx_i^t)\\
        = & \grad f^T_{\sB_i^t}(\vx_i^t)\mG_{m,t}^{-\frac{1}{4}}\left[\mG_{m,t}^{\frac{1}{4}} \left(\mG_{m,t}^{-\frac{1}{2}}-\mG_{i,t}^{-\frac{1}{2}}\right)\mG_{m,t}^{\frac{1}{4}}\right]\left[\mG_{m,t}^{\frac{1}{4}}\left(\mG_{m,t}^{-\frac{1}{2}}-\mG_{i,t}^{-\frac{1}{2}}\right)\mG_{m,t}^{\frac{1}{4}}\right]\mG_{m,t}^{-\frac{1}{4}}\grad f_{\sB_i^t}(\vx_i^t) \\
        =&\grad f^T_{\sB_i^t}(\vx_i^t)\mG_{m,t}^{-\frac{1}{4}}\left[\mG_{m,t}^{\frac{1}{4}}\mG_{i,t}^{-\frac{1}{2}}\mG_{m,t}^{\frac{1}{4}}-\mI\right]^2\mG_{m,t}^{-\frac{1}{4}}\grad f_{\sB_i^t}(\vx_i^t)\\
        \le & \lambda^2_{max}\left(\mG_{m,t}^{\frac{1}{4}}\mG_{i,t}^{-\frac{1}{2}}\mG_{m,t}^{\frac{1}{4}}-\mI\right)\lambda^{-\frac{1}{2}}_{min}\left(\mG_{m,t}\right)\left\|\grad f_{\sB_i^t}(\vx_i^t)\right\|^2 \mathop{\le}^{\circled{1}} \frac{\Delta_{1,t}G^2}{\lambda^{1.5}_{min}\left(\mG_{1,t}\right)}
    \end{aligned}
\end{equation}
\begin{equation}
    \label{ineq:T2_for_SD_final}
    \begin{split}
        T_2\le \frac{5\eta_{.,t}m\Delta_{1,t}G^2}{4\lambda^{1.5}_{min}\left(\mG_{1,t}\right)}.
    \end{split}
\end{equation}
\begin{equation}
    \label{ineq:T3_for_SD_component1}
    \begin{aligned}[b]
        &\eta_{.,t}\le \frac{\sqrt{\delta_{m,1}}}{4mL}\le \frac{\lambda_{min}\left(\mG^{\frac{1}{2}}_{m,1}\right)}{4mL}\le \frac{\lambda_{min}\left(\mG^{\frac{1}{2}}_{m,t}\right)}{4mL}  \Rightarrow \eta_{.,t}\mI \preceq \frac{\mG^{\frac{1}{2}}_{m,t}}{4mL} \mathop{\Rightarrow}^{\circled{1}} L\eta_{.,t}^2\mG^{-1}_{m,t} \preceq \frac{\eta_{.,t}}{4m}\mG_{m,t}^{-\frac{1}{2}}\\
        \Rightarrow & \left(\sum_{i=1}^m \grad f_{\sB_i^t}(\vx_i^t)\right)^T L\eta_{.,t}^2\mG^{-1}_{m,t}\left(\sum_{i=1}^m \grad f_{\sB_i^t}(\vx_i^t)\right) \le \left(\sum_{i=1}^m\grad f_{\sB_i^t}(\vx_i^t)\right)^T \frac{\eta_{.,t}}{4m}\mG_{m,t}^{-\frac{1}{2}}\left(\sum_{i=1}^m\grad f_{\sB_i^t}(\vx_i^t)\right),
    \end{aligned}
\end{equation}
\begin{equation}
    \label{ineq:comb_gradient_norm_upper_bound_LHS_1}
    \begin{aligned}[b]
        &\frac{c_{\sigma}m}{12Gc_{\kappa}\sqrt{nd}}\cdot\frac{1}{\sqrt{i}}\left\|\sum_{j=1}^m \grad f_{\sB_j^i}(\vx_j^i)\right\| \mathop{\le}^{\circled{1}} \frac{1}{2\sqrt{2}Gc_{\kappa}}\sqrt{\frac{\delta_{m,i}-\delta_{m,i-1}}{d}}\cdot\frac{1}{\sqrt{i}}\left\|\sum_{j=1}^m \grad f_{\sB_j^i}(\vx_j^i)\right\|\\
        = &\sqrt{\frac{\delta_{m,i}-\delta_{m,i-1}}{4im^2G^2d}}\frac{m}{\sqrt{2}c_{\kappa}}\left\|\sum_{j=1}^m \grad f_{\sB_j^i}(\vx_j^i)\right\| \\
        \mathop{\le}^{\circled{2}} &\sqrt{\frac{\delta_{m,i}-\delta_{m,i-1}}{4im^2G^2d}} \left[\sum_{j=1}^m \grad f_{\sB_j^i}(\vx_j^i)\right]^T \left(\mG_{m,i}-\mG_{m,i-1}\right)^{-\frac{1}{2}}\left[\sum_{j=1}^m \grad f_{\sB_j^i}(\vx_j^i)\right]\\
        \mathop{\le}^{\circled{3}} &\left(\sum_{j=1}^m \grad f_{\sB_j^i}(\vx_j^i)\right)^T\mG_{m,i}^{-\frac{1}{2}}\left(\sum_{j=1}^m \grad f_{\sB_i^j}(\vx_i^j)\right),
    \end{aligned}
\end{equation}
